# Supplementary material for: First measurement of $\eta$ production in neutrino interactions on argon with MicroBooNE
Source: arXiv:2305.16249 ancillary file (2024-05-04)
Supplement: Supplementary file 1 [file ETA_PRL_SUPPLEMENTARY_0524023_nolinenumbers.pdf]

# Supplementary Material: First measurement of $\eta$ production in neutrino interactions on argon with MicroBooNE

## I. SHOWER ENERGY-SCALE CALIBRATION, AND $\pi^0$ BACKGROUND CONSTRAINT.

Diphoton pairs from background  $\pi^0$  candidates can be isolated by requiring the reconstructed diphoton invariant mass be consistent with the  $\pi^0$  mass. The invariant mass is defined as

$$M_{\gamma\gamma} = \sqrt{2E_1E_2(1 - \cos\theta_{\gamma\gamma})}, \quad (1)$$

with  $E_1$  and  $E_2$  the energy of the leading and sub-leading photons, respectively, and  $\theta_{\gamma\gamma}$  the opening angle between the two photons. To select  $\pi^0$  candidates a requirement that  $M_{\gamma\gamma}$  be less than  $250 \text{ MeV}/c^2$  is imposed. The sample of events, referred to as the “ $\pi^0$ -sideband”, can be used to further validate the EM shower energy-scale calibration. The shape-only comparison of the data/MC agreement in the invariant diphoton mass for this sample of events is shown in Fig. 1. The background-subtracted  $M_{\gamma\gamma}$  distribution is fit to a Gaussian plus low-end exponential tail distribution to obtain a fit for the invariant mass of  $128 \text{ MeV}$  with a Gaussian width of  $31 \text{ MeV}$ . The energy of all EM showers is increased by  $5.2\%$  to correct for the difference between the measured and actual  $\pi^0$  mass. The same  $\pi^0$ -sideband will later be used to constrain  $\pi^0$  backgrounds in the cross section extraction.

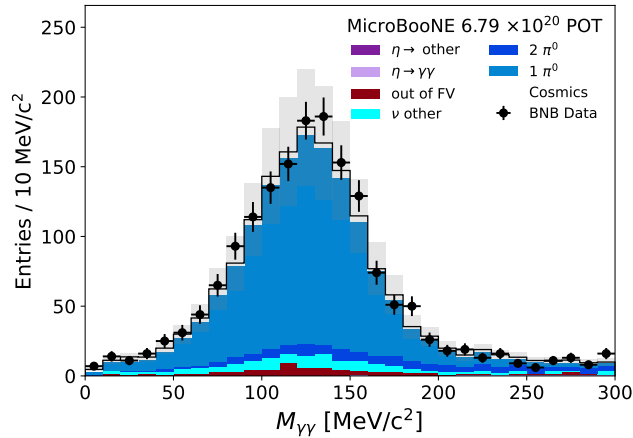

FIG. 1. Shape-only diphoton invariant mass from candidate  $\pi^0$  events.

Backgrounds to the analysis are primarily due to events with final-state  $\pi^0$ , with multi- $\pi^0$  events making the dominant background contribution. The background rate for  $1\pi^0$  and multi- $\pi^0$  events are constrained via in-situ measurement in sideband channels. For background events with a single final-state  $\pi^0$ , the  $\pi^0$ -sideband described above is used. For multi- $\pi^0$  events, the same  $\pi^0$ -sideband selection is applied but requiring four rather than two reconstructed showers greater than  $50 \text{ MeV}$  in energy and allowing  $M_{\gamma\gamma} < 700 \text{ MeV}$ . Backgrounds are constrained through the Conditional Covariance formalism [1] accounting for correlations between the sideband constraint sample and signal region. This method is used to update the predicted background rate and its uncertainty through the expressions below:

$$N_{MC}^{S, \text{constrained}} = N_{MC}^S + \frac{\sigma^{corr}}{(\sigma^B)^2} \times (N_{data}^B - N_{MC}^B), \quad (2)$$

$$(\sigma^{S, \text{constrained}})^2 = (\sigma^S)^2 - \frac{(\sigma^{corr})^2}{(\sigma^B)^2} \quad (3)$$

where  $N^{S,B}$  and  $\sigma^{S,B}$  are the number of events and their uncertainty; the superscripts  $B$  and  $S$  refer to events in the background constraint and signal region, respectively, and  $\sigma^{corr}$  refers to the covariance between background events measured in the constraint sideband and signal region. The measured correlation strength for  $1\pi^0$  and multi- $\pi^0$  sidebands and their expected rates in the signal region are  $0.73$  and  $0.79$ , respectively. The constraint procedure leads to an updated background rate in the signal region of  $13.2 \text{ } 1\pi^0$  and  $24.6 \text{ multi-}\pi^0$  events.

## II. $\eta$ SELECTION

To further reject background events with final-state  $\pi^0$  particles, two cuts on the kinematics of the diphoton pair are implemented:  $\cos\theta_{\gamma\gamma} < 0.5$  and  $M_{\min} > 400$  MeV/c<sup>2</sup>. The efficacy of this cut can be seen in Fig. 2. The plot shows the correlation between the sum of the shower energy and the diphoton opening angle for both  $\eta$  and  $\pi^0$  decays. The black and blue dotted lines trace the value of  $M_{\min}$  as a function of the true minimum opening angle kinematically allowed by the decay. The red points show the correlation between the two variables for reconstructed  $\eta \rightarrow \gamma\gamma$  decays from the simulation, while the tiled 2D histogram shows the same reconstructed distribution for true  $\pi^0 \rightarrow \gamma\gamma$  events. The figure shows both how  $\pi^0$  decays are much more boosted due to the lower  $\pi^0$  mass for equal energy photon pairs. This motivates the cut at  $\cos\theta_{\gamma\gamma} < 0.5$  which removes a very small amount of signal  $\eta$  candidates. The strong separation in 2D between the two distributions further justifies the cut on  $M_{\min}$  which can nicely separate the two populations as indicated by the dotted curves that trace the profile of  $M_{\min}$  for the values of  $M_{\min}$  equal to the  $\pi^0$  and  $\eta$  mass.

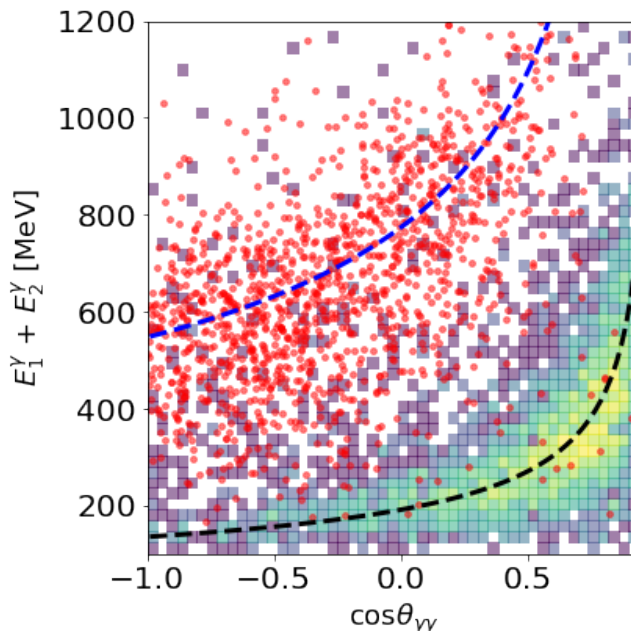

FIG. 2. Discrimination of  $\eta$  and  $\pi^0$  events decaying to two photons based on diphoton kinematics. The black and blue dotted lines trace the value of  $M_{\min}$  as a function of the true minimum opening angle kinematically allowed by the decay. The red points show the correlation between the two variables for reconstructed  $\eta \rightarrow \gamma\gamma$  decays from the simulation, while the tiled 2D histogram shows the same reconstructed distribution for true  $\pi^0 \rightarrow \gamma\gamma$  events from the simulation.

Figures 3 and 4 show the distributions of  $M_{\min}$  and  $\cos\theta_{\gamma\gamma}$  before cuts on these variables are applied. The plots show the clear separation between signal  $\eta$  events in purple and background. Cut values for these variables were determined by studying the prediction only distribution from simulation without information on the distribution of data events.

Figure 5 shows the efficiency for selecting  $\eta$  candidates for the different selection stages in the analysis. At every step in the selection, the efficiency is flat with respect to the  $\eta$  particle's energy, up to 1 GeV. After implementing a requirement that two reconstructed showers with greater than 50 MeV of energy each are reconstructed in the event, the efficiency drops to 40%, a consequence largely of reconstruction inefficiencies in events with complex topologies with multiple EM showers. Further quality cuts on the reconstructed showers bring the efficiency to 20%, while the rejection of  $\pi^0$  candidates through the cut  $M_{\gamma\gamma} > 250$  MeV has negligible impact on the efficiency. The final selection requirement that  $M_{\min} > 400$  MeV and  $\cos\theta_{\gamma\gamma} < 0.5$  decreases the efficiency to 13.6% without, however, energy-dependence up to 1 GeV.

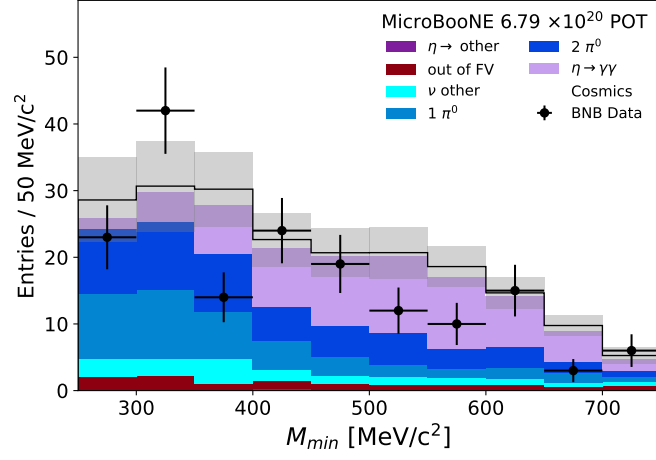

FIG. 3. Distribution for  $M_{\min}$  before the final selection cuts on this variable and  $\cos\theta_{\gamma\gamma}$  are applied.

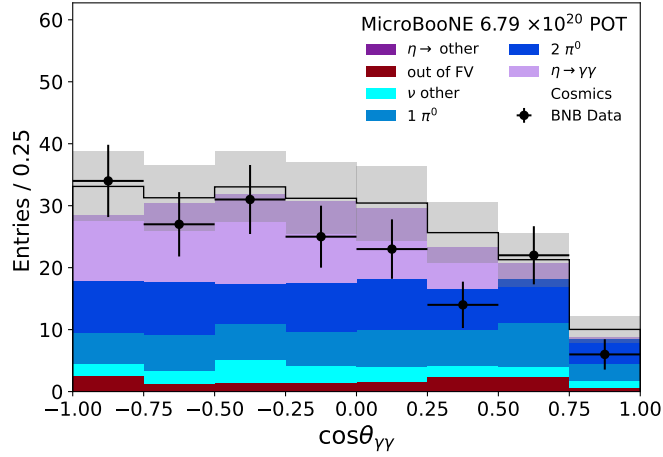

FIG. 4. Distribution for  $\cos\theta_{\gamma\gamma}$  before the final selection cuts on this variable and  $M_{\min}$  are applied.

### III. EXTRACTED CROSS SECTION

Figure 6 shows a comparison of the extracted flux-integrated cross section to that obtained through truth-studies of different generators. The result here is presented for inclusive  $\eta$  production after having corrected for the branching ratio for  $\eta \rightarrow 2\gamma$  of  $39.41\% \pm 0.20\%$  [2]. Note that the very high precision with which this branching ratio is measured does not introduce a noticeable increase in the uncertainty in the extracted cross section. The extracted cross section of  $3.22 \pm 0.84$  (stat.)  $\pm 0.86$  (syst.)  $10^{-41} \text{cm}^2/\text{nucleon}$ . The measurement from NEUT [3] of  $1.19 \cdot 10^{-40} \text{cm}^2/\text{nucleon}$ , found to be significantly larger than the extracted cross section, falls out of range of the plot above.

The limited nucleon excitations that decay with sizeable branching ratios to  $\eta$  particles leads to the observation that selecting  $\eta$  candidates is a powerful way to tag specific resonance states. In particular, nearly 90% of  $\eta$  particles produced in neutrino interactions from the BNB in MicroBooNE are predicted to originate from the decay of the  $N(1535)$  excitation. Figure 7 shows a truth-level distribution of the hadronic invariant mass  $W$  from the GENIE v3.0.6 G18.10a.02.11a generator prediction for MicroBooNE's neutrino flux for resonant interactions separated by each resonant state.  $\Delta(1232)$  dominates the resonant production. The contribution from the  $N(1535)$ , subleading with respect to the  $\Delta$ , is significant compared to other less relevant resonances. While the  $N(1520)$  has a comparable contribution to the event rate, its branching ratio to  $\eta$  mesons is negligible. The clear separation in the invariant mass due to the excitation is something that was observed with the  $\eta$  candidates from the analysis, as presented in the main results for the analysis.

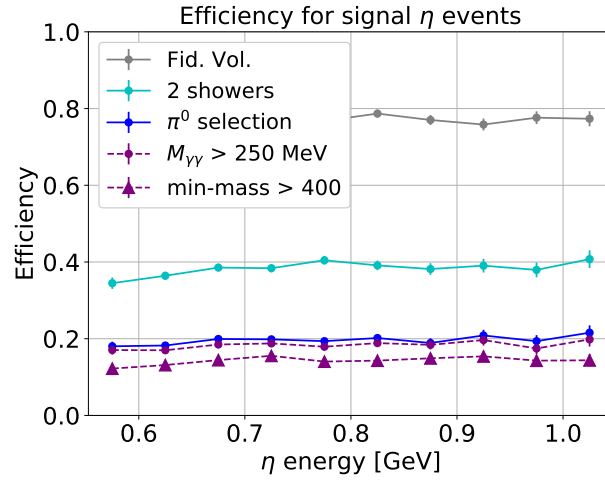

FIG. 5.  $\eta$  selection efficiency. The grey curve labeled as “Fid. Vol.” denotes the efficiency for identifying a neutrino interaction which match the signal topology within the MicroBooNE fiducial volume.

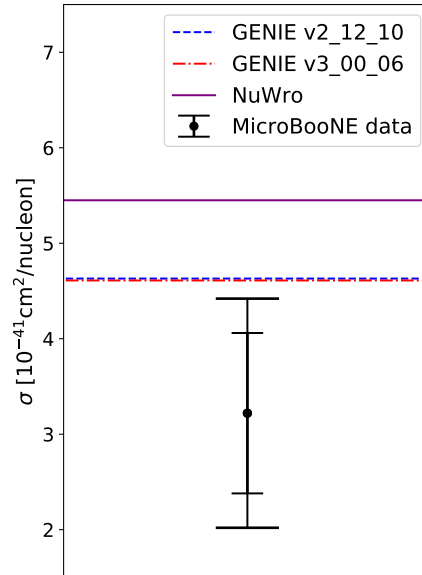

FIG. 6. Comparison of extracted cross section from data to predictions.

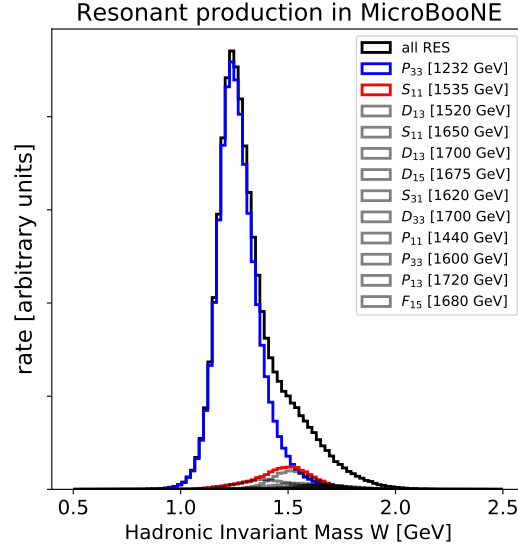

FIG. 7. Comparison of extracted cross section from data to predictions. The resonance labeled as  $P_{33}$  (blue) corresponds to the  $\Delta(1232)$ , and  $S_{11}$  (red) corresponds to  $N(1535)$ . The state  $D_{13}$  corresponds to the  $N(1520)$  resonance.

- 
- [1] Morris L. Eaton, *Multivariate statistics: a vector space approach* (Wiley, New York, 1983) pp. 116–117.
  - [2] R. L. Workman and Others (Particle Data Group), “Review of Particle Physics,” PTEP **2022**, 083C01 (2022).
  - [3] Yoshinari Hayato, “A neutrino interaction simulation program library NEUT,” Acta Phys. Polon. B **40**, 2477–2489 (2009).
